# Supplementary material for: On 4d rank-one N=3 superconformal field theories
Source: arXiv:1602.01503 ancillary file (2016-02-03)
Supplement: Supplementary file 1 [file chiralAlgebra.pdf]

---

## Setting up

In this notebook we construct the 2d chiral algebras associated to 4d rank-1  $N=3$  SCFTs. Note that within this notebook what is referred by script  $\mathcal{I}$  is denoted by  $k$ . We use the *Mathematica* code “SOPEN2defs” developed by Krivonos and Thielemans [hep-th/9512029]. It can be obtained from one of its authors K. Thielemans (k.thielemans@ucl.ac.uk). We assume it is saved in the same directory/folder as this notebook.

```
SetDirectory[NotebookDirectory[]];
```

```
<< SOPEN2defs.m
```

```
SOPEN2defs Version 1. (beta 2) by Kris Thielemans and Sergey Krivonos
```

```
Type ?SOPEN2defsHelp for a primer on SOPEN2defs (try it !).
```

As the helpful output of SOPEN2defs are sometimes annoying, we disable it:

```
Unprotect[Print]; Print[_] := {}; Protect[Print];
```

First we set up the OPE of the super energy-momentum tensor multiplet. This is done by first declaring the symbol to be used, and then listing the residues of the poles under  $Z_{12}$  using MakeOPE:

```
Bosonic[J]
```

```
OPE[J, J] =
```

```
MakeOPE[{c / 3 One + t12 ** tb12 ** J, tb12 ** DBT[J] - t12 ** DT[J] + t12 ** tb12 ** J' }]
```

```
<< 2 || |  $\frac{c \text{ One}}{3} + t_{12} ** tb_{12} ** J$  || 1 ||
```

```
- t12 ** DT[J] + tb12 ** DBT[J] + t12 ** tb12 ** J' >>
```

Here,  $t_{12}$  is  $\theta_{12}$ ,  $tb_{12}$  is  $\bar{\theta}_{12}$ ,  $DT$  is the superderivative  $D$ , and  $DBT$  is  $\bar{D}$ .  $D\bar{D}$  which is  $[D, \bar{D}]$ , will also be used below. Later it will be useful to have a function to extract the coefficients of  $\theta_{12}$  etc:

```
coeffOf t12 tb12 [x_] := x /. NonCommutativeMultiply[t12, tb12, y_] -> y
```

```
coeffOf t12 [x_] := coeffOf t12 tb12 [tb12 ** x]
```

```
coeffOf tb12 [x_] := coeffOf t12 tb12 [t12 ** x]
```

```
coeffOf 1 [x_] := coeffOf t12 tb12 [t12 ** tb12 ** x]
```

---

## $k=3$

Let us first consider the case  $k=3$ .

A superprimary has the following OPE in general:

```
primaryope[op_] := MakeOPE[{ $\Delta[op]$  t12 ** tb12 ** op,  
- F[op] op - t12 ** DT[op] + tb12 ** DBT[op] + t12 ** tb12 ** op' }]
```

Here we declare that  $W$  and  $\bar{W}$  (denoted as  $WB$  below) are a chiral primary and an antichiral primary with the required dimensions. Note that somehow Krivonos and Thielemans defined (anti)chirality oppositely from the usual convention.

```
ACHiralBosonic[W];  $\Delta[W] = 3 / 2$ ; F[W] = 3;
```

```
ChiralBosonic[WB];  $\Delta[WB] = 3 / 2$ ; F[WB] = -3;
```

**OPE[J, W] = primaryope[W] // OPESimplify**

$$\ll 2 || \frac{3 \text{ t12} ** \text{tb12} ** W}{2} || 1 || -3 W - \text{t12} ** \text{DT}[W] + \text{t12} ** \text{tb12} ** W' \gg$$

**OPE[J, WB] = primaryope[WB] // OPESimplify**

$$\ll 2 || \frac{3 \text{ t12} ** \text{tb12} ** WB}{2} || 1 || 3 WB + \text{tb12} ** \text{DBT}[WB] + \text{t12} ** \text{tb12} ** WB' \gg$$

Now we set up the OPE of W and WB. As discussed in the paper, it should have the following form:

**OPE[W, WB] = MakeOPE[{(3/2) a t12 \*\* tb12 \*\* One,  
a One + (2/2) t12 \*\* tb12 \*\* J,  
J + t12 \*\* DT[J]  
+ (1/2) t12 \*\* tb12 \*\* (u1 NO[J, J] + u2 DDB[J] + u3 J'),  
u1 NO[J, J] + u2 DDB[J] + u3 J'  
+ t12 \*\* DT[u1 NO[J, J] + u2 DDB[J] + u3 J']}] // OPESimplify;**

We fix the coefficients by demanding that the Jacobi identity for J, W and WB be satisfied. The failure is given by:

**OPEJacobi[J, W, WB, Function → Factor] // Union**

$$\left\{ 0, \frac{1}{3} (9a + c) \text{One}, \frac{1}{6} J (9 + 2cu1 - 6u2), \frac{1}{3} J (9 + 2cu1 - 6u2), \right. \\ \frac{1}{12} \text{One} (-9a + 2cu1 - 6cu2), \frac{1}{6} \text{One} (-9a + 2cu1 - 6cu2), \frac{2}{3} J (6 + cu1 - 3u2 - 3u3), \\ \frac{1}{2} J (-1 + 2u3), J (-1 + 2u3), \frac{1}{6} \text{One} (9a + 2cu3), \frac{1}{3} \text{One} (9a + 2cu3), \\ \frac{1}{3} \text{One} (18a - cu1 + 3cu2 + 3cu3), \frac{1}{2} (u1 - 3u2 + u3) \text{DBT}[J], (u1 - 3u2 + u3) \text{DBT}[J], \\ \frac{1}{2} (1 + u1 - 3u2 - u3) \text{DT}[J], (1 + u1 - 3u2 - u3) \text{DT}[J], (-2 - u1 + 3u2 + 3u3) \text{DT}[J], \\ \left. \frac{1}{3} (6 - 3u1 + 2cu1 + 3u2 + 3u3) \text{DT}[J], \frac{1}{2} (-u1 + 3u2 - u3) \text{DDB}[J] + \frac{1}{2} (u1 - 3u2 + u3) J' \right\}$$

Here and below, it is useful to ignore numerical coefficients before the terms that should vanish. So let us define a function to remove them:

**Prune[x\_] := PruneItem /@ x**

**PruneItem[x\_] := x**

**PruneItem[Times[n\_?NumberQ, xs\_]] := Times[xs]**

Then the failure of the Jacobi is given by

**OPEJacobi[J, W, WB, Function → Factor] // Prune // Union**

$$\left\{ 0, (9a + c) \text{One}, J (9 + 2cu1 - 6u2), \text{One} (-9a + 2cu1 - 6cu2), J (6 + cu1 - 3u2 - 3u3), \right. \\ J (-1 + 2u3), \text{One} (9a + 2cu3), \text{One} (18a - cu1 + 3cu2 + 3cu3), \\ (u1 - 3u2 + u3) \text{DBT}[J], (1 + u1 - 3u2 - u3) \text{DT}[J], (-2 - u1 + 3u2 + 3u3) \text{DT}[J], \\ \left. (6 - 3u1 + 2cu1 + 3u2 + 3u3) \text{DT}[J], \frac{1}{2} (-u1 + 3u2 - u3) \text{DDB}[J] + \frac{1}{2} (u1 - 3u2 + u3) J' \right\}$$

which is much shorter. All terms can be made zero by the following choice:

**solution = Solve[GetCoefficients[%] == 0]**

$$\left\{ \left\{ a \rightarrow -\frac{c}{9}, u1 \rightarrow -\frac{4}{-1+c}, u2 \rightarrow \frac{-9+c}{6(-1+c)}, u3 \rightarrow \frac{1}{2} \right\} \right\}$$

As explained in Krivonos-Thielemans, we then need to check the Jacobi for every permutation:

```
(OPEJacobi@@#) & /@Permutations[{J, W, WB}] /. solution[[1]] // Simplify //
Flatten // Union
{0}
```

Good. Then we demand the Jacobi of W, W and WB to vanish:

```
OPEJacobi[W, W, WB, Function -> Factor] /. solution[[1]] // Simplify // Prune // Union
{0, (15 + c) W / (-1 + c), (15 + c) DT[W] / (-1 + c),
  DT[W'] - NO[J, DT[W]] + 3 NO[DT[J], W] / (-1 + c), NO[DT[J], DT[W]] / (-1 + c)}
```

The terms proportional to W can be made to vanish only when  $c = -15$ . We also see that we need to set the following operator as null:

```
null = DT[W'] - NO[J, DT[W]] + 3 NO[DT[J], W]; Δ>null = 3; F>null = 2;
```

Now we study the Jacobi for all permutations of W, W and WB:

```
(OPEJacobi@@#) & /@Permutations[{W, W, WB}] /. solution[[1]] /.
{c -> -15, DT[W'] -> Expand[DT[W'] - null]} // Simplify // Flatten // Union
{0, -2 NO[DT[J], DT[W]],
  1/4 (-2 NO[J, W'] + 2 NO[DBT[J], DT[W]] + 3 NO[DDB[J], W] + 3 NO[J', W] + 2 W'')}
```

The reminders are both descendants of null, as you can easily see:

```
DT>null / 2
```

```
-2 NO[DT[J], DT[W]]
```

```
2 DBT>null // Simplify
```

```
2 NO[J, W'] - 2 NO[DBT[J], DT[W]] - 3 NO[DDB[J], W] - 3 NO[J', W] - 2 W''
```

We also need to check that the OPE of the null field with J, W, WB only produces operators with larger or equal dimensions. First we can check that this null field is a super Virasoro primary:

```
OPE[J, null] - primaryope>null /. solution[[1]] /.
{c -> -15, DT[W'] -> Expand[DT[W'] - null]} // Simplify
```

```
<< >>
```

Second its OPE with W vanishes:

```
OPE[W, null] /. solution[[1]] /. {c -> -15, DT[W'] -> Expand[DT[W'] - null]} // Simplify
```

```
<< >>
```

Finally its OPE with WB is:

```

OPE[WB, null] /. solution[[1]] /.
{c → -15, DT[W'] → Expand[DT[W'] - null]} // Simplify
<< 2 | |
1
8 (12 tb12 ** DDB[J'] + 12 tb12 ** NO[J, DDB[J]] + 2 tb12 ** NO[J, NO[J, J]] - 72 tb12 **
NO[W, WB] + 12 tb12 ** NO[DBT[J], DT[J]] + 18 tb12 ** NO[J', J] + 14 tb12 ** J'' + 6
tb12 ** tb12 ** DT[J''] + t12 ** tb12 ** NO[J, NO[J, DT[J]]] + 3 t12 ** tb12 ** NO[DDB
[J], DT[J]] - 12 t12 ** tb12 ** NO[DT[W], WB] + 4 t12 ** tb12 ** NO[DT[J'], J] +
2 t12 ** tb12 ** NO[J', DT[J]]) | | 1 | |
1
12 (-18 DT[J''] - 3 NO[J, NO[J, DT[J]]] - 9 NO[DDB[J], DT[J]] + 36 NO[DT[W], WB] - 12
NO[DT[J'], J] - 6 NO[J', DT[J]] + 9 tb12 ** DDB[J''] - 3 tb12 ** NO[J, NO[J, DDB[J]]
] - 12 tb12 ** NO[J, NO[DBT[J], DT[J]]] - 72 tb12 ** NO[W, WB'] + 6 tb12 ** NO[
DDB[J'], J] - 24 tb12 ** NO[DT[W], DBT[WB]] + 9 tb12 ** NO[J', DDB[J]] + 3 tb12
** NO[J', NO[J, J]] + 15 tb12 ** NO[J', J'] + 12 tb12 ** NO[J'', J] + 13 tb12 ** J(3))
>>

```

It only consists of operators with dimensions larger than that of the original null field. In particular, the coefficient of  $\bar{\theta}_{12}$  of the leading pole is

```

relation = coeffOf tb12 [OPEPole[2] [%]] // Expand
3 DDB[J'] / 2 + 3 / 2 NO[J, DDB[J]] + 1 / 4 NO[J, NO[J, J]] -
9 NO[W, WB] + 3 / 2 NO[DBT[J], DT[J]] + 9 / 4 NO[J', J] + 7 J'' / 4

```

which automatically realizes the expected Higgs branch relation  $J^3 \sim W \bar{W}$ . Including the coefficients, we have  $J^3/4 = 9 W \bar{W}$  up to descendants.

## An aside

Let us reproduce the results of Odake and Inami-Matsuo-Yamanaka, where almost the same problem was analyzed; they took the bottom components of  $W$  and  $\bar{W}$  to be fermionic, probably because fields with half-integral spin was assumed to be so. As OPEdefs do not like operators with the same name with different Grassmann assignment, we call them  $Z$  and  $ZB$ :

```

AChiralFermionic[Z]; Δ[Z] = 3 / 2; F[Z] = 3;
ChiralFermionic[ZB]; Δ[ZB] = 3 / 2; F[ZB] = -3;
OPE[J, Z] = primaryope[Z] // OPESimplify;
OPE[J, ZB] = primaryope[ZB] // OPESimplify;

```

The OPE of  $Z$  and  $ZB$  should be exactly as before:

```

OPE[Z, ZB] = MakeOPE[{(3 / 2) a t12 ** tb12 ** One,
a One + (2 / 2) t12 ** tb12 ** J,
J + t12 ** DT[J]
+ (1 / 2) t12 ** tb12 ** (u1 NO[J, J] + u2 DDB[J] + u3 J')},
u1 NO[J, J] + u2 DDB[J] + u3 J'
+ t12 ** DT[u1 NO[J, J] + u2 DDB[J] + u3 J']] /. solution[[1]] // OPESimplify;

```

Just to be sure, let's check the Jacobi:

```
(OPEJacobi@@#) & /@Permutations[{J, Z, ZB}] // Simplify // Flatten // Union
{0}
```

Good. The the Jacobi of Z, Z and ZB gives

```
OPEJacobi[Z, Z, ZB, Function → Factor] // Factor // Prune // Union
{0,  $\frac{(-9+c)Z}{-1+c}$ ,  $\frac{(-9+c)DT[Z]}{-1+c}$ ,  $\frac{-27DT[Z'] + cDT[Z'] - 18NO[J, DT[Z]] - 18NO[DT[J], Z]}{-1+c}$ ,  $\frac{-18NO[J, Z] - 27Z' + cZ'}{-1+c}$ }
```

We see we need to set c=9, as was shown in old papers:

```
OPEJacobi[Z, Z, ZB, Function → Factor] /. c → 9 // Factor // Prune // Union
{0, DT[Z'] + NO[J, DT[Z]] + NO[DT[J], Z], NO[J, Z] + Z'}
```

The null field in this case should be

```
nullF = NO[J, Z] + Z'; Δ>nullF] = 5 / 2; F>nullF] = 3;
```

The Jacobi identities in other permutations give:

```
(OPEJacobi@@#) & /@Permutations[{Z, Z, ZB}] /. {c → 9, Z' → Expand[Z' - nullF],
Z'' → Expand[Z' - nullF]'} // Factor // Flatten // Prune // Union
{0, NO[DBT[J], Z], 2 NO[DBT[J], DT[Z]] - NO[DDB[J], Z] + NO[J', Z]}
```

We see that the remainders are indeed descendants of the null field:

```
DBT>nullF]
```

```
NO[DBT[J], Z]
```

```
DDB>nullF] /. {Z' → Expand[Z' - nullF], Z'' → Expand[Z' - nullF]'} // Simplify
-2 NO[DBT[J], DT[Z]] + NO[DDB[J], Z] - NO[J', Z]
```

The null field is super Virasoro primary as before:

```
OPE[J, nullF] - primaryope>nullF] /. c → 9 // Simplify
```

```
<< >>
```

And the OPE with Z and ZB only gives higher-dimension fields:

```
OPE[Z, nullF] // Simplify
```

```
<< 1 || 2 t12 ** NO[Z, DT[Z]] >>
```

```
OPE[ZB, nullF] /. c → 9 // Simplify
```

```
<< 2 ||
 $\frac{1}{4}$  (t12 ** tb12 ** NO[J, NO[J, J]] - 6 t12 ** tb12 ** NO[Z, ZB] - 3 t12 ** tb12 ** NO[J', J]
+ t12 ** tb12 ** J'') || 1 ||
 $\frac{1}{2}$  (-NO[J, NO[J, J]] + 6 NO[Z, ZB] + 3 NO[J', J] - 2 tb12 ** NO[J, NO[J, DBT[J]]] - 4
tb12 ** NO[Z, DBT[ZB]] + 2 tb12 ** NO[J', DBT[J]] - J'') >>
```

Before analyzing  $k = 4$  and  $6$ , it is instructive to consider the case  $k=2$ . First let's clear the internal state of OPEdefs:

```
ClearOPESavedValues[]
```

We redefine the charges as appropriate for  $k = 2$  :

```
 $\Delta[W] = 1; F[W] = 2;$ 
```

```
OPE[J, W] = primaryope[W] // OPESimplify
```

```
<< 2 || t12 ** tb12 ** W || 1 || -2 W - t12 ** DT[W] + t12 ** tb12 ** W' >>
```

```
 $\Delta[WB] = 1; F[WB] = -2;$ 
```

```
OPE[J, WB] = primaryope[WB] // OPESimplify
```

```
<< 2 || t12 ** tb12 ** WB || 1 || 2 WB + tb12 ** DBT[WB] + t12 ** tb12 ** WB' >>
```

The  $W - WB$  OPE is very simple:

```
OPE[W, WB] = MakeOPE[{(2/2) a t12 ** tb12 ** One,
  a One + (1/2) t12 ** tb12 ** J,
  J + t12 ** DT[J]
}];
```

The Jacobi for  $J, W, WB$  immediately fixes the coefficients.

```
OPEJacobi[J, W, WB, Function -> Factor] // Prune // Union
```

```
{0, (6 a + c) One}
```

```
OPE[W, WB] = MakeOPE[{(2/2) a t12 ** tb12 ** One,
  a One + (1/2) t12 ** tb12 ** J,
  J + t12 ** DT[J]
}] /. a -> -c/6 // OPESimplify
```

```
<< 3 || -1/6 c t12 ** tb12 ** One || 2 ||
  -c One/6 + t12 ** tb12 ** J/2 || 1 || J + t12 ** DT[J] >>
```

```
ClearOPESavedValues[]
```

```
(OPEJacobi@@#) & /@ Permutations[{J, W, WB}] // Simplify // Flatten // Union
{0}
```

And then the Jacobi for  $W, W$  and  $WB$  is automatically satisfied, as it should be.

```
(OPEJacobi@@#) & /@ Permutations[{W, W, WB}] // Simplify // Flatten // Union
{0}
```

Now let us demand that there is a relation of the form  $W \overline{W} \sim J^2$ . The most general form is

```
op = NO[W, WB] + a NO[J, J] + b J' + d DDB[J];  $\Delta[op] = 2; F[op] = 0;$ 
```

We demand that it is a super Virasoro primary :

```
OPE[J, op] - primaryope[op] // GetCoefficients // Simplify
```

```
{1/6 c (-1 + 2 a - 6 d), 1/3 (c + 2 b c), 1 + 2 b, 2 a c/3 - 2 (1 + d), -1 + a - b - 3 d, a + b - 3 d}
```

```
solution = Solve[% == 0, {a, b, d}]
```

$$\left\{ \left\{ a \rightarrow \frac{5}{2(-1+c)}, b \rightarrow -\frac{1}{2}, d \rightarrow -\frac{-6+c}{6(-1+c)} \right\} \right\}$$

```
op = op /. solution[[1]]
```

$$-\frac{(-6+c) \text{DDB}[J]}{6(-1+c)} + \frac{5 \text{NO}[J, J]}{2(-1+c)} + \text{NO}[W, WB] - \frac{J'}{2}$$

Its OPE with W is

```
OPE[W, op] // FullSimplify
```

$$\begin{aligned} & \ll 3 \mid - \frac{(-6+c)(9+c) \text{t12} ** \text{tb12} ** W}{6(-1+c)} \mid 2 \mid \\ & \frac{1}{6(-1+c)} (9+c) (-(-6+c) W + 3 \text{t12} ** \text{tb12} ** \text{NO}[J, W] + 3 \text{t12} ** \text{tb12} ** W') \mid 1 \mid \\ & \frac{1}{3(-1+c)} (3(9+c) \text{NO}[J, W] + (3+2c) \text{t12} ** \text{DT}[W'] + 3(5 \text{t12} ** \text{NO}[J, \text{DT}[W]] + (-1+c) \\ & \quad \text{t12} ** \text{NO}[\text{DT}[J], W] + (9+c) W')) \gg \end{aligned}$$

from which we immediately see that we need  $c=-9$  or  $+6$  for the “op” not to force  $W$  itself to be zero. When  $c=+6$ , we also see  $JW + (\text{descendants})=0$ , which we do not want. So we conclude that in order to just impose the relation  $W \overline{W} \sim J^2$ , we are required to take  $c=-9$ , and this is the value that follows from the 4d analysis. The final relation then is

```
op = op /. c -> -9
```

$$-\frac{\text{DDB}[J]}{4} - \frac{1}{4} \text{NO}[J, J] + \text{NO}[W, WB] - \frac{J'}{2}$$

So the relation is  $J^2 = 4W \overline{W}$  up to descendants.

## k=4

Now let us proceed to  $k=4$ .

```
ClearOPESavedValues[]
```

It would be convenient to have a function that generates all possible operators of a given dimension constructed out of  $J$  only. A quick hack is as follows :

$$\begin{aligned} \mathbf{x} = & (1 - \mathbf{t} J) (1 - \mathbf{t}^2 J') (1 - \mathbf{t}^3 J'') (1 - \mathbf{t}^4 J''') (1 - \mathbf{t}^5 J'''' ) (1 - \mathbf{t}^6 J''''') \\ & (1 - \mathbf{t}^{(3/2)} \mathbf{q} \text{DT}[J]) (1 - \mathbf{t}^{(5/2)} \mathbf{q} \text{DT}[J']) (1 - \mathbf{t}^{(7/2)} \mathbf{q} \text{DT}[J'']) * \\ & (1 - \mathbf{t}^{(3/2)} \mathbf{q}^{(-1)} \text{DBT}[J]) (1 - \mathbf{t}^{(5/2)} \mathbf{q}^{(-1)} \text{DBT}[J']) \\ & (1 - \mathbf{t}^{(7/2)} \mathbf{q}^{(-1)} \text{DBT}[J'']) * \\ & (1 - \mathbf{t}^2 \text{DDB}[J]) (1 - \mathbf{t}^3 \text{DDB}[J']) (1 - \mathbf{t}^4 \text{DDB}[J'']) \\ & (1 - \mathbf{t}^5 \text{DDB}[J''']) (1 - \mathbf{t}^6 \text{DDB}[J'''']); \end{aligned}$$

```
XX = 1 / X + O[t]^7 // Normal;
```

```
monom[n_] := MonomialList[Residue[Coefficient[XX, t^n] / q, {q, 0}]]
```

```
NOy[x_] := x; NOy[x__] := NO[x];
```

```
monomToNO[{x__}] := NOy @@ (Join @@ (monomToNOx /@ {x}));
```

```
monomToNO[x_] := monomToNO[{x}];
```

```

monomToNOX[Power[x_, n_]] := Table[x, n];
monomToNOX[x_] := {x};
SetOPEOptions[NOOrdering, 1];
ops[n_] := ops[n] = monomToNO /@ (monom[n] /. Times → List)

```

We can test it:

```

ops[1]
{J}

ops[2]
{NO[J, J], DDB[J], J'}

ops[3]
{NO[J, NO[J, J]], NO[J, DDB[J]], NO[J, J'], DDB[J'], NO[DBT[J], DT[J]], J''}

```

Then the following gives a generic linear combination of dimension- $n$  composite operators constructed of J:

```

gL[n_, a_] := Sum[ops[n][[i]] a[i], {i, 1, Length[ops[n]]}

```

Now we set the dimensions of W and WB as appropriate for  $k=4$ :

```

 $\Delta[W] = 2; F[W] = 4;$ 
OPE[J, W] = primaryope[W] // OPESimplify
<< 2 || 2 t12 ** tb12 ** W || 1 || -4 W - t12 ** DT[W] + t12 ** tb12 ** W' >>

 $\Delta[WB] = 2; F[WB] = -4;$ 
OPE[J, WB] = primaryope[WB] // OPESimplify
<< 2 || 2 t12 ** tb12 ** WB || 1 || 4 WB + tb12 ** DBT[WB] + t12 ** tb12 ** WB' >>

```

The OPE of W and WB has the general form

```

OPE[W, WB] = MakeOPE[{(4 / 2) a t12 ** tb12 ** One,
  a One + (3 / 2) t12 ** tb12 ** J,
  J + t12 ** DT[J]
  + (2 / 2) t12 ** tb12 ** gL[2, A],
  gL[2, A] + t12 ** DT[gL[2, A]]
  + (1 / 2) t12 ** tb12 ** gL[3, AA],
  gL[3, AA] + t12 ** DT[gL[3, AA]]}] // OPESimplify;

```

from which we can fix the coefficients by demanding the J-W-WB Jacobi:

```

OPEJacobi[J, W, WB, Function → Factor] // Union;

```



**solution = Solve[GetCoefficients[%] == 0]**

$$\left\{ \left\{ a \rightarrow -\frac{c}{12}, A[1] \rightarrow -\frac{11}{2(-1+c)}, A[2] \rightarrow \frac{-12+c}{6(-1+c)}, A[3] \rightarrow \frac{1}{2}, \right. \right.$$

$$AA[1] \rightarrow \frac{9(29+4c)}{18-27c+7c^2+2c^3}, AA[2] \rightarrow \frac{396+63c-8c^2}{2(18-27c+7c^2+2c^3)},$$

$$AA[3] \rightarrow -\frac{11}{2(-1+c)}, AA[4] \rightarrow \frac{-324-9c-9c^2+c^3}{6(18-27c+7c^2+2c^3)},$$

$$\left. AA[5] \rightarrow \frac{-288+36c-c^2}{18-27c+7c^2+2c^3}, AA[6] \rightarrow \frac{-270+9c+6c^2+2c^3}{6(18-27c+7c^2+2c^3)} \right\}$$

**(OPEJacobi@@#) &/@Permutations[{J, W, WB}] /. solution[[1]] // Simplify //**  
**Flatten // Union**  
 {0}

We then move on to the Jacobi of W, W and WB:

**remainder =**

**OPEJacobi[W, W, WB, Function → Factor] /. solution[[1]] // Factor // Prune // Union**

$$\left\{ 0, \frac{(-12+c)(9+c)(21+c)W}{(-1+c)(6+c)(-3+2c)}, \frac{(-12+c)(9+c)(21+c)DT[W]}{(-1+c)(6+c)(-3+2c)}, \right.$$

$$\left( (9+c) \left( -1476 DT[W'] - 99c DT[W'] + 2c^2 DT[W'] - 2052 NO[J, DT[W]] - 27c NO[J, DT[W]] + \right. \right.$$

$$\left. 648 NO[DT[J], W] - 252c NO[DT[J], W] \right) / ((-1+c)(6+c)(-3+2c)),$$

$$\left( (9+c) \left( -1188 DT[W'] - 12c DT[W'] + c^2 DT[W'] - 576 NO[J, DT[W]] - \right. \right.$$

$$\left. 51c NO[J, DT[W]] - 1476 NO[DT[J], W] + 24c NO[DT[J], W] \right) /$$

$$((-1+c)(6+c)(-3+2c)), \frac{(-12+c)(9+c)NO[DT[J], DT[W]]}{(-1+c)(6+c)(-3+2c)},$$

$$\left( -522 NO[J, NO[DT[J], DT[W]]] - 72c NO[J, NO[DT[J], DT[W]]] - 846 NO[DT[J], DT[W']] - \right.$$

$$69c NO[DT[J], DT[W']] + 2c^2 NO[DT[J], DT[W']] + 162 NO[DT[J'], DT[W]] +$$

$$42c NO[DT[J'], DT[W]] + 5c^2 NO[DT[J'], DT[W]] \Big) / ((-1+c)(6+c)(-3+2c)),$$

$$\left( -1692 DT[W''] - 138c DT[W''] + 4c^2 DT[W''] + 648 NO[J, DT[W']] - 6c NO[J, DT[W']] - \right.$$

$$4c^2 NO[J, DT[W']] + 1044 NO[J, NO[J, DT[W]]] + 144c NO[J, NO[J, DT[W]]] -$$

$$4176 NO[J, NO[DT[J], W]] - 576c NO[J, NO[DT[J], W]] + 360 NO[DDB[J], DT[W]] +$$

$$30c NO[DDB[J], DT[W]] - 5c^2 NO[DDB[J], DT[W]] - 9504 NO[DT[J], W'] -$$

$$834c NO[DT[J], W'] + 20c^2 NO[DT[J], W'] + 1296 NO[DT[J'], W] + 336c NO[DT[J'], W] +$$

$$40c^2 NO[DT[J'], W] + 36 NO[J', DT[W]] - 54c NO[J', DT[W]] - 15c^2 NO[J', DT[W]] \Big) /$$

$$((-1+c)(6+c)(-3+2c)), \frac{(9+c)(21+c)(-36 NO[J, W] - 48 W' + c W')}{(-1+c)(6+c)(-3+2c)} \}$$

We do not study all the possibilities; for now let us content ourselves with the fact that the value  $c=-21$ , which is expected from the 4d analysis, is an allowed value at this point. Let us further study the Jacobi identity by setting  $c$  to this value:

```

remainder =
  OPEJacobi[W, W, WB, Function → Factor] /. solution[[1]] /. c → -21 // Factor //
  Prune // Union
{0, -DT[W'] + NO[J, DT[W]] - 4 NO[DT[J], W],
  DT[W'] - NO[J, DT[W]] + 4 NO[DT[J], W], NO[DT[J], DT[W]],
  2 NO[J, NO[DT[J], DT[W]]] + 3 NO[DT[J], DT[W']] + 3 NO[DT[J'], DT[W]],
  6 DT[W''] - 2 NO[J, DT[W']] - 4 NO[J, NO[J, DT[W]]] + 16 NO[J, NO[DT[J], W]] -
  5 NO[DDB[J], DT[W]] + 34 NO[DT[J], W'] + 24 NO[DT[J'], W] - 11 NO[J', DT[W]],
  -6 DT[W''] + 2 NO[J, DT[W']] + 4 NO[J, NO[J, DT[W]]] - 16 NO[J, NO[DT[J], W]] +
  5 NO[DDB[J], DT[W]] - 34 NO[DT[J], W'] - 24 NO[DT[J'], W] + 11 NO[J', DT[W]]}

```

So we need the following null field:

```

null = DT[W'] - NO[J, DT[W]] + 4 NO[DT[J], W]; Δ[null] = 7 / 2; F[null] = 3;

```

Note that it has the following descendant:

```

DT[null]

```

```

-5 NO[DT[J], DT[W]]

```

```

DBT[null]

```

```

NO[J, W'] - NO[DBT[J], DT[W]] + 4  $\left(-\frac{1}{2} \text{NO}[DDB[J], W] - \frac{1}{2} \text{NO}[J', W]\right) - W''$ 
```

```

null' / 5 /. W'' → W'' + DBT[null] // Expand

```

```

 $-\frac{1}{2} \text{NO}[DDB[J], DT[W]] + \text{NO}[DT[J], W'] - \frac{1}{2} \text{NO}[J', DT[W]]$ 

```

So we can set up the following rule killing some of the null fields:

```

nullRules = {DT[W'] → DT[W'] - null, DT[W''] → DT[W''] - null',
  NO[DT[J], DT[W]] → 0, W'' → W'' + DBT[null], W''' → W''' + DBT[null]',
  NO[DT[J], W'] → NO[J', DT[W]] / 2 + NO[DDB[J], DT[W]] / 2};

```

Then the Jacobi is now satisfied:

```

(OPEJacobi@@#) & /@Permutations[{W, W, WB}] /. solution[[1]] /. c → -21 //.
  nullRules // Factor // Flatten // Union
{0}

```

Note also that the OPE of the null field with J, W, WB contains operators with higher dimensions only:

```

OPE[J, null] - primaryope[null] /. solution[[1]] /. c → -21 // Simplify

```

```

<< >>

```

```

OPE[W, null] /. solution[[1]] /. c → -21 // Simplify

```

```

<< >>

```

**OPE[WB, null] /. solution[[1]] /. c → -21 // Simplify**

```
<< 2 | |
1
360 (252 tb12 ** DDB[J''] + 504 tb12 ** NO[J, DDB[J']] + 216 tb12 ** NO[J, NO[J, DDB[J]]]
    + 12 tb12 ** NO[J, NO[J, NO[J, J]]] + 288 tb12 ** NO[J, NO[J, J']] + 288 tb12
    ** NO[J, NO[DBT[J], DT[J]]] + 552 tb12 ** NO[J, J''] - 5760 tb12 ** NO[W, WB] +
    144 tb12 ** NO[DBT[J], DT[J']] + 144 tb12 ** NO[DDB[J], DDB[J]] + 432 tb12 ** NO[
    DDB[J], J'] - 432 tb12 ** NO[DT[J], DBT[J']] + 324 tb12 ** NO[J', J'] + 600 tb12
    ** J^(3) + 107 t12 ** tb12 ** DT[J^(3)] + 153 t12 ** tb12 ** NO[J, DT[J'']] + 54 t12 **
    tb12 ** NO[J, NO[J, DT[J']]] + 6 t12 ** tb12 ** NO[J, NO[J, NO[J, DT[J]]]] + 72
    t12 ** tb12 ** NO[J, NO[DDB[J], DT[J]]] + 54 t12 ** tb12 ** NO[J, NO[DT[J], J']] +
    72 t12 ** tb12 ** NO[DDB[J], DT[J']] + 72 t12 ** tb12 ** NO[DT[J], DDB[J']] + 42 t12
    ** tb12 ** NO[DT[J], J''] - 720 t12 ** tb12 ** NO[DT[W], WB] + 90 t12 ** tb12 ** NO[
    DT[J'], J']) || 1 | |
1
360 (-214 DT[J^(3)] - 3 (102 NO[J, DT[J'']] + 36 NO[J, NO[J, DT[J']]]) + 4 NO[J, NO[J, NO[
    J, DT[J]]]] + 48 NO[J, NO[DDB[J], DT[J]]] + 36 NO[J, NO[DT[J], J']] + 48
    NO[DDB[J], DT[J']] + 48 NO[DT[J], DDB[J']] + 28 NO[DT[J], J''] - 480 NO[DT[W],
    WB] + 60 NO[DT[J'], J'] - 72 tb12 ** DDB[J^(3)] - 87 tb12 ** NO[J, DDB[J'']] - 30
    tb12 ** NO[J, NO[J, DDB[J']]] + 6 tb12 ** NO[J, NO[J, NO[J, DDB[J]]]] - 6 tb12
    ** NO[J, NO[J, NO[J, J']]] + 24 tb12 ** NO[J, NO[J, NO[DBT[J], DT[J]]]] - 48
    tb12 ** NO[J, NO[J, J'']] + 12 tb12 ** NO[J, NO[DBT[J], DT[J']]] + 12 tb12 ** NO
    [J, NO[DDB[J], DDB[J]]] - 72 tb12 ** NO[J, NO[DDB[J], J']] + 12 tb12 ** NO[
    J, NO[DT[J], DBT[J']]] - 120 tb12 ** NO[J, NO[J', J']] - 159 tb12 ** NO[J,
    J^(3)] + 1440 tb12 ** NO[W, WB'] + 72 tb12 ** NO[DBT[J], DT[J'']] + 96 tb12 ** NO
    [DBT[J], NO[DDB[J], DT[J]]] - 48 tb12 ** NO[DBT[J'], DT[J']] - 48 tb12 ** NO
    [DDB[J], DDB[J']] - 84 tb12 ** NO[DDB[J], J''] - 192 tb12 ** NO[DDB[J'], J'] +
    48 tb12 ** NO[DT[J], DBT[J'']] + 360 tb12 ** NO[DT[W], DBT[WB]] - 258 tb12 ** NO
    [J', J''] - 137 tb12 ** J^(4)) >>
```

In particular, the last OPE means that the following WB descendant of the null field gives the Higgs branch relation:

**relation = coeffOf tb12 [OPEPole[2][%]] // Expand**

```
7 DDB[J'']
10
+ 7
5 NO[J, DDB[J']] + 3
5 NO[J, NO[J, DDB[J]]] +
1
30 NO[J, NO[J, NO[J, J]]] + 4
5 NO[J, NO[J, J']] + 4
5 NO[J, NO[DBT[J], DT[J]]] +
23
15 NO[J, J''] - 16 NO[W, WB] + 2
5 NO[DBT[J], DT[J']] + 2
5 NO[DDB[J], DDB[J]] +
6
5 NO[DDB[J], J'] - 6
5 NO[DT[J], DBT[J']] + 9
10 NO[J', J'] + 5 J^(3)
3
```

So the relation is  $J^2/30 = 16W\overline{W}$  up to descendants.

## k=6

The analysis for k=6 is entirely analogous, although more tedious.

**ClearOPESavedValues[]**

**Δ[W] = 3; F[W] = 6;**

```

OPE[J, W] = primaryope[W] // OPESimplify
<< 2 || 3 t12 ** tb12 ** W || 1 || -6 W - t12 ** DT[W] + t12 ** tb12 ** W' >>

Δ[WB] = 3; F[WB] = -6;

OPE[J, WB] = primaryope[WB] // OPESimplify
<< 2 || 3 t12 ** tb12 ** WB || 1 || 6 WB + tb12 ** DBT[WB] + t12 ** tb12 ** WB' >>

```

The OPE of W and WB has the general form

```

OPE[W, WB] = MakeOPE[{(6/2) a t12 ** tb12 ** One,
  a One + (5/2) t12 ** tb12 ** J,
  J + t12 ** DT[J]
  + (4/2) t12 ** tb12 ** gL[2, A],
  gL[2, A] + t12 ** DT[gL[2, A]]
  + (3/2) t12 ** tb12 ** gL[3, AA],
  gL[3, AA] + t12 ** DT[gL[3, AA]]
  + (2/2) t12 ** tb12 ** gL[4, AAA],
  gL[4, AAA] + t12 ** DT[gL[4, AAA]]
  + (1/2) t12 ** tb12 ** gL[5, AAAA],
  gL[5, AAAA] + t12 ** DT[gL[5, AAAA]]}] // OPESimplify;

```

from which we can fix the coefficients by demanding the J-W-WB Jacobi:

```
OPEJacobi[J, W, WB, Function → Factor] // Union;
```

```
solution = Solve[GetCoefficients[%] == 0];
```

We then move on to the Jacobi of W, W and WB:

```

remainder =
  OPEJacobi[W, W, WB, Function → Factor] /. solution[[1]] // Factor // Prune // Union;
{remainder[[2]], remainder[[3]]}
{
  
$$\frac{(-18 + c)(15 + c)(33 + c)(-135 - 153c + c^2)W}{(-1 + c)(1 + c)(6 + c)(-3 + 2c)(-9 + 5c)},$$

  
$$\left( \frac{(-18 + c)(15 + c)(33 + c)(8424 + 12528c - 138c^2 - 4c^3 + c^4)W}{((-2 + c)(-1 + c)(1 + c)(6 + c)(12 + c)(-3 + 2c)(-9 + 5c))} \right) \}$$

```

PolynomialGCD[-135 - 153 c + c<sup>2</sup>, 8424 + 12 528 c - 138 c<sup>2</sup> - 4 c<sup>3</sup> + c<sup>4</sup>]

1

We see that c=-33, -15, 18 are allowed at this point. We just consider the case c=-33. Now, to speed up the computation, we redefine the basic OPEs with the determined values:

```
ClearOPESavedValues[]
```

```

OPE[J, J] = MakeOPE[{c/3 One + t12 ** tb12 ** J,
  tb12 ** DBT[J] - t12 ** DT[J] + t12 ** tb12 ** J'}] /. c → -33;

```

```

OPE[W, WB] = MakeOPE[{(6/2) a t12 ** tb12 ** One,
  a One + (5/2) t12 ** tb12 ** J,
  J + t12 ** DT[J]
  + (4/2) t12 ** tb12 ** gL[2, A],
  gL[2, A] + t12 ** DT[gL[2, A]]
  + (3/2) t12 ** tb12 ** gL[3, AA],
  gL[3, AA] + t12 ** DT[gL[3, AA]]
  + (2/2) t12 ** tb12 ** gL[4, AAA],
  gL[4, AAA] + t12 ** DT[gL[4, AAA]]
  + (1/2) t12 ** tb12 ** gL[5, AAAA],
  gL[5, AAAA] + t12 ** DT[gL[5, AAAA]]}] /. solution[[1]] /. c -> -33 //
OPESimplify;

remainder = OPEJacobi[W, W, WB, Function -> Factor] // Factor // Prune // Union;

remainder[[2]]
-DT[W'] + NO[J, DT[W]] - 6 NO[DT[J], W]

```

So we need the following null field:

```
null = DT[W'] - NO[J, DT[W]] + 6 NO[DT[J], W]; Δ>null = 9/2; F>null = 5;
```

The Jacobi identity for W, W, WB now follows if we use the following descendants. There should be a more systematic way to carry it out, but for now we just enumerate them in an ad hoc manner.

First, the null field itself and its  $\bar{D}$  leads to the following basic rules:

```

DBT>null // Expand
NO[J, W'] - NO[DBT[J], DT[W]] - 3 NO[DDB[J], W] - 3 NO[J', W] - W''

basicRules = {DT[W'] -> DT[W'] - null,
  W'' -> W'' + DBT>null, W''' -> W''' + DBT>null',
  W'''' -> W'''' + DBT>null'', W''''' -> W''''' + DBT>null'''} // Expand;

```

Second, the  $D$  of the null field and its repeated derivatives lead to more rules:

```

DT>null
-7 NO[DT[J], DT[W]]

DT>null' // Expand
-7 NO[DT[J], DT[W']] - 7 NO[DT[J'], DT[W]]

DT>null'' //. basicRules // Expand
-7 NO[J, NO[J, NO[DT[J], DT[W]]]] +  $\frac{49}{2}$  NO[DDB[J], NO[DT[J], DT[W]]] +
 $\frac{35}{2}$  NO[DT[J], NO[J', DT[W]]] +  $\frac{35}{4}$  NO[DT[J''], DT[W]]

```

**DT[null]''' //. basicRules // Expand**

$$\begin{aligned}
& -7 \text{NO}[J, \text{NO}[J, \text{NO}[J, \text{NO}[\text{DT}[J], \text{DT}[W]]]]] + 49 \text{NO}[J, \text{NO}[\text{DDB}[J], \text{NO}[\text{DT}[J], \text{DT}[W]]]] + \\
& 28 \text{NO}[J, \text{NO}[\text{DT}[J], \text{NO}[J', \text{DT}[W]]]] + 14 \text{NO}[J, \text{NO}[\text{DT}[J''], \text{DT}[W]]] + \\
& \frac{49}{2} \text{NO}[\text{DDB}[J], \text{NO}[\text{DT}[J'], \text{DT}[W]]] + \frac{49}{2} \text{NO}[\text{DT}[J], \text{NO}[\text{DDB}[J'], \text{DT}[W]]] + \\
& 49 \text{NO}[\text{DT}[J], \text{NO}[\text{DT}[J'], W']] - 7 \text{NO}[\text{DT}[J], \text{NO}[J'', \text{DT}[W]]] + \\
& \frac{49}{2} \text{NO}[\text{DT}[J'], \text{NO}[J', \text{DT}[W]]] + \frac{119}{12} \text{NO}[\text{DT}[J^{(3)}], \text{DT}[W]]
\end{aligned}$$

**DBT[DT[null]] //. basicRules // Expand**

$$\frac{7}{2} \text{NO}[\text{DDB}[J], \text{DT}[W]] - 7 \text{NO}[\text{DT}[J], W'] + \frac{7}{2} \text{NO}[J', \text{DT}[W]]$$

**moreRules = {NO[DT[J], DT[W]] → 0,**

**NO[DT[J'''], DT[W]] → NO[DT[J'''], DT[W]] - 4 / 35 DT[null]''',**

**NO[DT[J'''], DT[W]] → NO[DT[J'''], DT[W]] - 12 / 119 DT[null]''',**

**NO[DT[J], W'] → NO[DT[J], W'] + DBT[DT[null]] / 7} //. basicRules // Expand;**

At this point the failure of the Jacobi are not very long:

**remainder =**

**(OPEJacobi@@#) & @Permutations[{W, W, WB}] //. Join[basicRules, moreRules] //**  
**Factor // Flatten // Prune // Union**

$$\begin{aligned}
& \{0, 58 \text{NO}[\text{DDB}[J], \text{NO}[\text{DT}[J'], \text{DT}[W]]] + \\
& 109 \text{NO}[\text{DT}[J], \text{NO}[\text{DDB}[J'], \text{DT}[W]]] + 116 \text{NO}[\text{DT}[J], \text{NO}[\text{DT}[J'], W']] - \\
& 87 \text{NO}[\text{DT}[J], \text{NO}[J'', \text{DT}[W]]] + 58 \text{NO}[\text{DT}[J'], \text{NO}[J', \text{DT}[W]]], \\
& -87 \text{NO}[\text{DDB}[J], \text{NO}[J', \text{DT}[W]]] + 48 \text{NO}[\text{DDB}[J''], \text{DT}[W]] + \\
& 192 \text{NO}[\text{DT}[J], \text{NO}[\text{DBT}[J'], \text{DT}[W]]] + 174 \text{NO}[\text{DT}[J], \text{NO}[J', W']] + \\
& 87 \text{NO}[\text{DT}[J''], W'] - 87 \text{NO}[J', \text{NO}[J', \text{DT}[W]]] - 74 \text{NO}[J^{(3)}, \text{DT}[W]], \\
& -54 \text{NO}[\text{DDB}[J], \text{NO}[J', \text{DT}[W]]] + 3 \text{NO}[\text{DDB}[J''], \text{DT}[W]] + \\
& 12 \text{NO}[\text{DT}[J], \text{NO}[\text{DBT}[J'], \text{DT}[W]]] + 108 \text{NO}[\text{DT}[J], \text{NO}[J', W']] + \\
& 54 \text{NO}[\text{DT}[J''], W'] - 54 \text{NO}[J', \text{NO}[J', \text{DT}[W]]] - 37 \text{NO}[J^{(3)}, \text{DT}[W]], \\
& 54 \text{NO}[\text{DDB}[J], \text{NO}[J', \text{DT}[W]]] - 3 \text{NO}[\text{DDB}[J''], \text{DT}[W]] - \\
& 12 \text{NO}[\text{DT}[J], \text{NO}[\text{DBT}[J'], \text{DT}[W]]] - 108 \text{NO}[\text{DT}[J], \text{NO}[J', W']] - \\
& 54 \text{NO}[\text{DT}[J''], W'] + 54 \text{NO}[J', \text{NO}[J', \text{DT}[W]]] + 37 \text{NO}[J^{(3)}, \text{DT}[W]], \\
& 87 \text{NO}[\text{DDB}[J], \text{NO}[J', \text{DT}[W]]] - 48 \text{NO}[\text{DDB}[J''], \text{DT}[W]] - \\
& 192 \text{NO}[\text{DT}[J], \text{NO}[\text{DBT}[J'], \text{DT}[W]]] - 174 \text{NO}[\text{DT}[J], \text{NO}[J', W']] - 87 \text{NO}[\text{DT}[J''], W'] + \\
& 87 \text{NO}[J', \text{NO}[J', \text{DT}[W]]] + 74 \text{NO}[J^{(3)}, \text{DT}[W]], 6 \text{NO}[\text{DBT}[J'], \text{NO}[J', \text{DT}[W]]] + \\
& 3 \text{NO}[\text{DBT}[J^{(3)}], \text{DT}[W]] + 6 \text{NO}[\text{DDB}[J], \text{NO}[\text{DBT}[J'], \text{DT}[W]]] + \\
& 3 \text{NO}[\text{DDB}[J''], W'] + 12 \text{NO}[\text{DT}[J], \text{NO}[\text{DBT}[J'], W']] - \text{NO}[J^{(3)}, W']\}
\end{aligned}$$

Finally, we need a few really ad hoc descendants to see that the remainders above are set to zero:

**A = DBT[DT[null] ''] // . basicRules // Simplify // Expand**

$$\begin{aligned} & \frac{7}{2} \text{NO}[J, \text{NO}[J, \text{NO}[\text{DDB}[J], \text{DT}[W]]]] - 7 \text{NO}[J, \text{NO}[J, \text{NO}[\text{DT}[J], W']]] + \\ & \frac{7}{2} \text{NO}[J, \text{NO}[J, \text{NO}[J', \text{DT}[W]]]] - 14 \text{NO}[J, \text{NO}[\text{DBT}[J], \text{NO}[\text{DT}[J], \text{DT}[W]]]] - \\ & \frac{49}{4} \text{NO}[\text{DDB}[J], \text{NO}[\text{DDB}[J], \text{DT}[W]]] + \frac{49}{2} \text{NO}[\text{DDB}[J], \text{NO}[\text{DT}[J], W']] - \\ & 21 \text{NO}[\text{DDB}[J], \text{NO}[J', \text{DT}[W]]] + \frac{7}{2} \text{NO}[\text{DDB}[J''], \text{DT}[W]] + \\ & 14 \text{NO}[\text{DT}[J], \text{NO}[\text{DBT}[J'], \text{DT}[W]]] + \frac{35}{2} \text{NO}[\text{DT}[J], \text{NO}[J', W']] + \\ & \frac{35}{4} \text{NO}[\text{DT}[J''], W'] - \frac{35}{4} \text{NO}[J', \text{NO}[J', \text{DT}[W]]] - 7 \text{NO}[J^{(3)}, \text{DT}[W]] \end{aligned}$$

**B = NO[J', DBT[DT[null]]] // . basicRules // Simplify // Expand**

$$\begin{aligned} & \frac{7}{2} \text{NO}[\text{DDB}[J], \text{NO}[J', \text{DT}[W]]] - 7 \text{NO}[\text{DT}[J], \text{NO}[J', W']] - \\ & \frac{7}{2} \text{NO}[\text{DT}[J''], W'] + \frac{7}{2} \text{NO}[J', \text{NO}[J', \text{DT}[W]]] + \frac{7}{3} \text{NO}[J^{(3)}, \text{DT}[W]] \end{aligned}$$

**evenMoreRules =**

**Solve[{A == 0, B == 0}, {NO[DT[J''], W'], NO[J^{(3)}, DT[W]]}]][1] // . basicRules // Expand**

$$\begin{aligned} & \{ \text{NO}[\text{DT}[J''], W'] \rightarrow 2 \text{NO}[J, \text{NO}[J, \text{NO}[\text{DDB}[J], \text{DT}[W]]]] - \\ & 4 \text{NO}[J, \text{NO}[J, \text{NO}[\text{DT}[J], W']]] + 2 \text{NO}[J, \text{NO}[J, \text{NO}[J', \text{DT}[W]]]] - \\ & 8 \text{NO}[J, \text{NO}[\text{DBT}[J], \text{NO}[\text{DT}[J], \text{DT}[W]]]] - 7 \text{NO}[\text{DDB}[J], \text{NO}[\text{DDB}[J], \text{DT}[W]]] + \\ & 14 \text{NO}[\text{DDB}[J], \text{NO}[\text{DT}[J], W']] - 6 \text{NO}[\text{DDB}[J], \text{NO}[J', \text{DT}[W]]] + 2 \text{NO}[\text{DDB}[J''], \text{DT}[W]] + \\ & 8 \text{NO}[\text{DT}[J], \text{NO}[\text{DBT}[J'], \text{DT}[W]]] - 2 \text{NO}[\text{DT}[J], \text{NO}[J', W']] + \text{NO}[J', \text{NO}[J', \text{DT}[W]]], \\ & \text{NO}[J^{(3)}, \text{DT}[W]] \rightarrow 3 \text{NO}[J, \text{NO}[J, \text{NO}[\text{DDB}[J], \text{DT}[W]]]] - \\ & 6 \text{NO}[J, \text{NO}[J, \text{NO}[\text{DT}[J], W']]] + 3 \text{NO}[J, \text{NO}[J, \text{NO}[J', \text{DT}[W]]]] - \\ & 12 \text{NO}[J, \text{NO}[\text{DBT}[J], \text{NO}[\text{DT}[J], \text{DT}[W]]]] - \frac{21}{2} \text{NO}[\text{DDB}[J], \text{NO}[\text{DDB}[J], \text{DT}[W]]] + \\ & 21 \text{NO}[\text{DDB}[J], \text{NO}[\text{DT}[J], W']] - \frac{21}{2} \text{NO}[\text{DDB}[J], \text{NO}[J', \text{DT}[W]]] + \\ & 3 \text{NO}[\text{DDB}[J''], \text{DT}[W]] + 12 \text{NO}[\text{DT}[J], \text{NO}[\text{DBT}[J'], \text{DT}[W]]] \} \end{aligned}$$

**S = NO[DDB[J], DT[null]'] // . Join[basicRules, moreRules, evenMoreRules] // Expand**

$$\begin{aligned} & -\frac{98}{17} \text{NO}[\text{DDB}[J], \text{NO}[\text{DT}[J'], \text{DT}[W]]] - \\ & \frac{98}{17} \text{NO}[\text{DT}[J], \text{NO}[\text{DDB}[J'], \text{DT}[W]]] - \frac{196}{17} \text{NO}[\text{DT}[J], \text{NO}[\text{DT}[J'], W']] + \\ & \frac{147}{17} \text{NO}[\text{DT}[J], \text{NO}[J'', \text{DT}[W]]] - \frac{98}{17} \text{NO}[\text{DT}[J'], \text{NO}[J', \text{DT}[W]]] \end{aligned}$$

**T = NO[DT[DDB[J]], null'] // . Join[basicRules, moreRules, evenMoreRules] // Expand**

$$\begin{aligned} & \frac{14}{17} \text{NO}[\text{DDB}[J], \text{NO}[\text{DT}[J'], \text{DT}[W]]] + \\ & \frac{147}{34} \text{NO}[\text{DT}[J], \text{NO}[\text{DDB}[J'], \text{DT}[W]]] + \frac{28}{17} \text{NO}[\text{DT}[J], \text{NO}[\text{DT}[J'], W']] - \\ & \frac{21}{17} \text{NO}[\text{DT}[J], \text{NO}[J'', \text{DT}[W]]] + \frac{14}{17} \text{NO}[\text{DT}[J'], \text{NO}[J', \text{DT}[W]]] \end{aligned}$$

```

furtherRules = Solve[{S == 0, T == 0},
  { NO[DT[J], NO[DT[J'], W]], NO[DT[J], NO[DDB[J'], DT[W]]] }][[1]]
{ NO[DT[J], NO[DT[J'], W']] →
   $\frac{1}{4} (-2 \text{ NO}[DDB[J], \text{ NO}[DT[J'], DT[W]]] + 3 \text{ NO}[DT[J], \text{ NO}[J'', DT[W]]] -$ 
   $2 \text{ NO}[DT[J'], \text{ NO}[J', DT[W]]]) , \text{ NO}[DT[J], \text{ NO}[DDB[J'], DT[W]]] → 0 \}$ 

DBT[B] 12 / 7 //. Join[basicRules, moreRules, evenMoreRules, furtherRules] // Expand
6 NO[DBT[J'], NO[J', DT[W]]] +
3 NO[DBT[J(3)], DT[W]] + 6 NO[DDB[J], NO[DBT[J'], DT[W]]] +
3 NO[DDB[J''], W'] + 12 NO[DT[J], NO[DBT[J'], W']] - NO[J(3), W']

finalRules = { NO[J(3), W'] → NO[J(3), W'] + DBT[B] 12 / 7 } //.
Join[basicRules, moreRules, evenMoreRules, furtherRules] // Expand
{ NO[J(3), W'] → 6 NO[DBT[J'], NO[J', DT[W]]] +
3 NO[DBT[J(3)], DT[W]] + 6 NO[DDB[J], NO[DBT[J'], DT[W]]] +
3 NO[DDB[J''], W'] + 12 NO[DT[J], NO[DBT[J'], W']] }

remainder //. Join[basicRules, moreRules, evenMoreRules,
  furtherRules, finalRules] // Factor // Flatten // Union
{ 0 }

```

Note also that the OPE of the null field with J, W, WB contains operators with higher dimensions only.

```
OPE[J, null] - primaryope[null] // Simplify
```

```
<< >>
```

```
OPE[W, null] // Simplify
```

```
<< >>
```

The OPE with WB is very long, so we do not show it explicitly

```
tmp = OPE[WB, null] // Simplify;
```

But we can check that its leading pole is of order 2,

```
MaxPole[tmp]
```

```
2
```

which guarantees that indeed there is no term with higher dimension than the null operator itself.

In fact the residue of this second order pole does not have a term without  $\theta$  or  $\bar{\theta}$ :

```
coeffOf1[OPEPole[2][tmp]]
```

```
0
```

The leading term in the OPE is the following WB descendant of the null field and it gives the Higgs branch relation:



**relation = coeffOf**tb12**[OPEPole[2][tmp]] // Expand**

$$\begin{aligned}
& \frac{229}{1344} \text{DDB}[J^{(4)}] + \frac{97}{252} \text{NO}[J, \text{DDB}[J^{(3)}]] + \frac{5}{21} \text{NO}[J, \text{NO}[J, \text{DDB}[J'']]] + \\
& \frac{2}{21} \text{NO}[J, \text{NO}[J, \text{NO}[J, \text{DDB}[J']]]] + \frac{5}{336} \text{NO}[J, \text{NO}[J, \text{NO}[J, \text{NO}[J, \text{DDB}[J]]]]] + \\
& \frac{\text{NO}[J, \text{NO}[J, \text{NO}[J, \text{NO}[J, \text{NO}[J, J]]]]]}{5040} + \frac{1}{56} \text{NO}[J, \text{NO}[J, \text{NO}[J, \text{NO}[J, J']]]] + \\
& \frac{1}{42} \text{NO}[J, \text{NO}[J, \text{NO}[J, \text{NO}[\text{DBT}[J], \text{DT}[J]]]]] + \frac{25}{252} \text{NO}[J, \text{NO}[J, \text{NO}[J, J'']]] + \\
& \frac{1}{14} \text{NO}[J, \text{NO}[J, \text{NO}[\text{DBT}[J], \text{DT}[J']]]] + \frac{3}{28} \text{NO}[J, \text{NO}[J, \text{NO}[\text{DDB}[J], \text{DDB}[J]]]] + \\
& \frac{15}{56} \text{NO}[J, \text{NO}[J, \text{NO}[\text{DDB}[J], J']]] - \frac{1}{7} \text{NO}[J, \text{NO}[J, \text{NO}[\text{DT}[J], \text{DBT}[J']]]] + \\
& \frac{19}{112} \text{NO}[J, \text{NO}[J, \text{NO}[J', J']]] + \frac{19}{48} \text{NO}[J, \text{NO}[J, J^{(3)}]] + \frac{25}{84} \text{NO}[J, \text{NO}[\text{DBT}[J], \text{DT}[J'']]] + \\
& \frac{3}{14} \text{NO}[J, \text{NO}[\text{DBT}[J], \text{NO}[\text{DDB}[J], \text{DT}[J]]]] + \frac{3}{14} \text{NO}[J, \text{NO}[\text{DBT}[J], \text{NO}[\text{DT}[J], J']]] + \\
& \frac{13}{42} \text{NO}[J, \text{NO}[\text{DBT}[J'], \text{DT}[J']]] + \frac{27}{56} \text{NO}[J, \text{NO}[\text{DDB}[J], \text{DDB}[J']]] + \\
& \frac{13}{28} \text{NO}[J, \text{NO}[\text{DDB}[J], J'']] + \frac{115}{168} \text{NO}[J, \text{NO}[\text{DDB}[J'], J']] - \\
& \frac{4}{21} \text{NO}[J, \text{NO}[\text{DT}[J], \text{DBT}[J'']]] + \frac{19}{28} \text{NO}[J, \text{NO}[J', J'']] + \frac{97}{180} \text{NO}[J, J^{(4)}] - \\
& 36 \text{NO}[W, WB] + \frac{89}{504} \text{NO}[\text{DBT}[J], \text{DT}[J^{(3)}]] + \frac{3}{28} \text{NO}[\text{DBT}[J], \text{NO}[\text{DDB}[J], \text{DT}[J']]] + \\
& \frac{3}{14} \text{NO}[\text{DBT}[J], \text{NO}[\text{DT}[J], \text{DDB}[J']]] + \frac{5}{28} \text{NO}[\text{DBT}[J], \text{NO}[\text{DT}[J], J'']] + \\
& \frac{11}{84} \text{NO}[\text{DBT}[J], \text{NO}[\text{DT}[J'], J']] + \frac{85}{168} \text{NO}[\text{DBT}[J'], \text{DT}[J'']] + \\
& \frac{31}{112} \text{NO}[\text{DDB}[J], \text{DDB}[J'']] + \frac{3}{56} \text{NO}[\text{DDB}[J], \text{NO}[\text{DDB}[J], \text{DDB}[J]]] + \\
& \frac{3}{14} \text{NO}[\text{DDB}[J], \text{NO}[\text{DDB}[J], J']] - \frac{9}{28} \text{NO}[\text{DDB}[J], \text{NO}[\text{DT}[J], \text{DBT}[J']]] + \\
& \frac{97}{336} \text{NO}[\text{DDB}[J], \text{NO}[J', J']] + \frac{13}{24} \text{NO}[\text{DDB}[J], J^{(3)}] + \\
& \frac{1}{4} \text{NO}[\text{DDB}[J'], \text{DDB}[J']] + \frac{1}{2} \text{NO}[\text{DDB}[J'], J''] - \frac{115}{504} \text{NO}[\text{DT}[J], \text{DBT}[J^{(3)}]] - \\
& \frac{29}{84} \text{NO}[\text{DT}[J], \text{NO}[\text{DBT}[J'], J']] - \frac{19}{84} \text{NO}[\text{DT}[J'], \text{DBT}[J'']] + \frac{53}{112} \text{NO}[J', \text{DDB}[J'']] + \\
& \frac{11}{84} \text{NO}[J', \text{NO}[J', J']] + \frac{13}{16} \text{NO}[J', J^{(3)}] + \frac{127}{504} \text{NO}[J'', J''] + \frac{1123}{4032} J^{(5)}
\end{aligned}$$

So the relation is  $J^2/5040 = 36W \overline{W}$  up to descendants.

## Anti-climactic aside: $k=5$

As a final exercise, let us show that the 2d chiral algebra for the would-be 4d  $N=3$   $k=5$  theory also exists.

**ClearOPESavedValues[]**

$\Delta[W] = 5/2$ ;  $F[W] = 5$ ;

```
OPE[J, W] = primaryope[W] // OPESimplify
```

```
<< 2 ||  $\frac{5 \text{ t12 ** tb12 ** W}}{2}$  || 1 || -5 W - t12 ** DT[W] + t12 ** tb12 ** W' >>
```

```
 $\Delta[\text{WB}] = 5/2$ ; F[WB] = -5;
```

```
OPE[J, WB] = primaryope[WB] // OPESimplify
```

```
<< 2 ||  $\frac{5 \text{ t12 ** tb12 ** WB}}{2}$  || 1 || 5 WB + tb12 ** DBT[WB] + t12 ** tb12 ** WB' >>
```

```
OPE[J, J] =
```

```
MakeOPE[{c / 3 One + t12 ** tb12 ** J, tb12 ** DBT[J] - t12 ** DT[J] + t12 ** tb12 ** J' }]
```

```
<< 2 ||  $\frac{c \text{ One}}{3} + \text{t12 ** tb12 ** J}$  || 1 ||  
-t12 ** DT[J] + tb12 ** DBT[J] + t12 ** tb12 ** J' >>
```

The OPE of W and WB has the general form

```
OPE[W, WB] = MakeOPE[{(5 / 2) a t12 ** tb12 ** One,  
a One + (4 / 2) t12 ** tb12 ** J,  
J + t12 ** DT[J]  
+ (3 / 2) t12 ** tb12 ** gL[2, A],  
gL[2, A] + t12 ** DT[gL[2, A]]  
+ (2 / 2) t12 ** tb12 ** gL[3, AA],  
gL[3, AA] + t12 ** DT[gL[3, AA]]  
+ (1 / 2) t12 ** tb12 ** gL[4, AAA],  
gL[4, AAA] + t12 ** DT[gL[4, AAA]]}] // OPESimplify;
```

from which we can fix the coefficients by demanding the J-W-WB Jacobi. Then we study the Jacobi for W, W, WB:

```
OPEJacobi[J, W, WB, Function → Factor] // Union;
```

```
solution = Solve[GetCoefficients[%] == 0];
```

```
remainder =
```

```
OPEJacobi[W, W, WB, Function → Factor] /. solution[[1]] // Factor // Prune // Union;
```

```
{remainder[[2]], remainder[[3]]}
```

```
{  $\frac{(27 + c) (-1008 - 99 c + c^2) W}{(-1 + c) (6 + c) (-3 + 2 c)}$ ,  $\frac{(27 + c) (33768 + 37395 c - 1469 c^2 - 95 c^3 + 9 c^4) W}{(-1 + c) (1 + c) (6 + c) (-3 + 2 c) (-9 + 5 c)}$  }
```

```
PolynomialGCD[-1008 - 99 c + c2, 33768 + 37395 c - 1469 c2 - 95 c3 + 9 c4]
```

```
1
```

We see that only  $c = -27$  is allowed at this point. Note that  $-27 = -3(2k-1)$ . Let us redefine the basic OPEs with the determined values:

```
ClearOPESavedValues[]
```

```
OPE[J, J] = MakeOPE[{c / 3 One + t12 ** tb12 ** J,  
tb12 ** DBT[J] - t12 ** DT[J] + t12 ** tb12 ** J' }] /. c → -27;
```

```

OPE[W, WB] = MakeOPE[{(5/2) a t12 ** tb12 ** One,
  a One + (4/2) t12 ** tb12 ** J,
  J + t12 ** DT[J]
  + (3/2) t12 ** tb12 ** gL[2, A],
  gL[2, A] + t12 ** DT[gL[2, A]]
  + (2/2) t12 ** tb12 ** gL[3, AA],
  gL[3, AA] + t12 ** DT[gL[3, AA]]
  + (1/2) t12 ** tb12 ** gL[4, AAA],
  gL[4, AAA] + t12 ** DT[gL[4, AAA]]}] /. solution[[1]] /. c -> -27 //
OPESimplify;

remainder = OPEJacobi[W, W, WB, Function -> Factor] // Factor // Prune // Union;

remainder[[2]]
- DT[W'] + NO[J, DT[W]] - 5 NO[DT[J], W]

So we need the following null field:

null = DT[W'] - NO[J, DT[W]] + 5 NO[DT[J], W]; Δ[null] = 4; F[null] = 4;

Necessaray descendants can be constructed completely analogously as was in k=6:

DBT[null] // Expand

NO[J, W'] - NO[DBT[J], DT[W]] -  $\frac{5}{2}$  NO[DDB[J], W] -  $\frac{5}{2}$  NO[J', W] - W''

basicRules = {DT[W'] -> DT[W'] - null,
  W' -> W' + DBT[null], W'' -> W'' + DBT[null]',
  W''' -> W''' + DBT[null]'', W'''' -> W'''' + DBT[null]'''} // Expand;

DT[null]
- 6 NO[DT[J], DT[W]]

DT[null]' // Expand
- 6 NO[DT[J], DT[W']] - 6 NO[DT[J'], DT[W]]

DT[null]'' // basicRules // Expand
- 6 NO[J, NO[J, NO[DT[J], DT[W]]]] + 18 NO[DDB[J], NO[DT[J], DT[W]]] +
  12 NO[DT[J], NO[J', DT[W]]] + 6 NO[DT[J''], DT[W]]

DT[null]''' // basicRules // Expand
- 6 NO[J, NO[J, NO[J, NO[DT[J], DT[W]]]]] +
  36 NO[J, NO[DDB[J], NO[DT[J], DT[W]]]] + 18 NO[J, NO[DT[J], NO[J', DT[W]]]] +
  9 NO[J, NO[DT[J''], DT[W]]] + 18 NO[DDB[J], NO[DT[J'], DT[W]]] +
  18 NO[DT[J], NO[DDB[J'], DT[W]]] + 36 NO[DT[J], NO[DT[J'], W']] -
  6 NO[DT[J], NO[J'', DT[W]]] + 18 NO[DT[J'], NO[J', DT[W]]] + 7 NO[DT[J(3)], DT[W]]

DBT[DT[null]] // basicRules // Expand
3 NO[DDB[J], DT[W]] - 6 NO[DT[J], W] + 3 NO[J', DT[W]]

moreRules = {NO[DT[J], DT[W]] -> 0,
  NO[DT[J'], DT[W]] -> NO[DT[J'], DT[W]] - 1/6 DT[null]'',
  NO[DT[J''], DT[W]] -> NO[DT[J''], DT[W]] - 1/7 DT[null]''',
  NO[DT[J], W'] -> NO[DT[J], W'] + DBT[DT[null]]/6} // basicRules // Expand;

```

We see that the Jacobi then vanishes:

```
remainder =
  (OPEJacobi@@#) & /@ Permutations[{W, W, WB}] /. Join[basicRules, moreRules] //
    Factor // Flatten // Prune // Union
{0}
```

Note also that the OPE of the null field with J, W, WB contains operators with higher dimensions only.

```
OPE[J, null] - primaryope[null] // Simplify
```

```
<< >>
```

```
OPE[W, null] // Simplify
```

```
<< >>
```

```
tmp = OPE[WB, null] // Simplify;
```

```
MaxPole[tmp]
```

```
2
```

The residue of this second order pole does not have a term without  $\theta$  or  $\bar{\theta}$ :

```
coeffOf1[OPEPole[2][tmp]]
```

```
0
```

The leading term in the OPE is the following WB descendant of the null field and it gives the Higgs branch relation:

```
relation = coeffOf1[OPEPole[2][tmp]] // Expand
```

$$\begin{aligned} & \frac{85}{168} \text{DDB}[J^{(3)}] + \frac{75}{112} \text{NO}[J, \text{DDB}[J'']] + \frac{55}{112} \text{NO}[J, \text{NO}[J, \text{DDB}[J']]] + \\ & \frac{5}{42} \text{NO}[J, \text{NO}[J, \text{NO}[J, \text{DDB}[J]]]] + \frac{1}{336} \text{NO}[J, \text{NO}[J, \text{NO}[J, \text{NO}[J, J]]]] + \\ & \frac{25}{168} \text{NO}[J, \text{NO}[J, \text{NO}[J, J']]] + \frac{5}{28} \text{NO}[J, \text{NO}[J, \text{NO}[\text{DBT}[J], \text{DT}[J]]]] + \\ & \frac{25}{48} \text{NO}[J, \text{NO}[J, J'']] + \frac{15}{56} \text{NO}[J, \text{NO}[\text{DBT}[J], \text{DT}[J']]] + \frac{75}{224} \text{NO}[J, \text{NO}[\text{DDB}[J], \text{DDB}[J]]] + \\ & \frac{25}{28} \text{NO}[J, \text{NO}[\text{DDB}[J], J']] - \frac{5}{8} \text{NO}[J, \text{NO}[\text{DT}[J], \text{DBT}[J']]] + \\ & \frac{135}{224} \text{NO}[J, \text{NO}[J', J']] + \frac{425}{336} \text{NO}[J, J^{(3)}] - 25 \text{NO}[W, \text{WB}] + \frac{65}{112} \text{NO}[\text{DBT}[J], \text{DT}[J'']] + \\ & \frac{25}{56} \text{NO}[\text{DBT}[J], \text{NO}[\text{DDB}[J], \text{DT}[J]]] + \frac{25}{56} \text{NO}[\text{DBT}[J], \text{NO}[\text{DT}[J], J']] + \\ & \frac{15}{28} \text{NO}[\text{DBT}[J'], \text{DT}[J']] + \frac{75}{112} \text{NO}[\text{DDB}[J], \text{DDB}[J']] + \frac{55}{84} \text{NO}[\text{DDB}[J], J''] + \\ & \frac{115}{112} \text{NO}[\text{DDB}[J'], J'] - \frac{5}{14} \text{NO}[\text{DT}[J], \text{DBT}[J'']] + \frac{25}{24} \text{NO}[J', J''] + \frac{16 J^{(4)}}{21} \end{aligned}$$

So the relation is  $J^2/336 = 25W \overline{W}$  up to descendants.

It seems that for general  $k$  we still have a corresponding 2d algebra at  $c = -3(2k-1)$  and the relation is

$$\frac{n!}{(2(n-1))!} J^2 = k^2 W \overline{W}$$

up to descendants.
